# Supplementary material for: Synthesis of Shared Control Protocols with Provable Safety and Performance Guarantees
Source: arXiv:1610.08500 source file (2016-10-26)
Supplement: Supplementary file 1 [file appendix.tex]

\clearpage
\appendix
\section{Appendix}\label{sec:appendix}

\subsection{Proofs}
\nj{Give formal proofs here.}

\subsection{Future Work}
\subsubsection{Transformation to a convex optimization problem}
\begin{newStuff}
In~\cite{boyd_convex_optimization}, it is described how a nonlinear program of a special form, called \emph{geometric program}, can be transformed into a convex optimization problem. We make use of this transformation.

\paragraph{Geometric programming}
Let $x=\{x_1,\ldots,x_n\}$ be a set of variables with variables $x_i\in\R_{>0}$ for $1\leq i\leq n$. Let $h(x)$ denote a \emph{monomial} over $x$ and $f(x)$ denote a \emph{posynomial} over $x$, as in~\cite{boyd_convex_optimization}. \nj{Add details.}

A \emph{geometric program} is of the form
\begin{align}
	\text{minimize} 		&\quad f_0(x)\\
	\text{such that} 		&\\
	\forall.\, 1\leq i\leq m 	&\quad f_i(x)\leq 1\\
	\forall.\, 1\leq i\leq p 	&\quad h_i(x)= 1
\end{align}
Summarized, only real-valued, positive variables are allowed. All posynomials are upper bounded by one, all monomials are equal to one, and the target function is a posynomial.

\paragraph{Transformation}
First, recall that in order for a nonlinear program to be geometrical, all variables need to be positive. 

For \emph{probability variables} $p_s$, we therefore have to ensure that the computed strategy ensures a positive reachability probability for target states. Algorithmically, this can be achieved by as a preprocessing in the following way: Compute the set of \emph{problematic states} for $\mdp_r$, \ie the set of states where a strategy exists that induces probability zero of reaching target states. For these states, inside the NLP encoding, reachability has to be ensured, see~\cite{wimmer-et-al-tcs-2014}.

For \emph{strategy variables} $\sched_{a}^{s,\act}$ and $\sched_{ha}^{s,\act}$, it is now no longer allowed to have probability zero for an action at state $s$, \ie $\sched_{a}^{s,\act}=0$ or $\sched_{ha}^{s,\act}=0$. We therefore ensure a \emph{minimal probability} $\p_\epsilon$ to be assigned for all actions at each state, \ie we have $\sched_{a}^{s,\act}\in[p_\epsilon,1]$ for $p_\epsilon\in [0,1]$

What to do about \emph{perturbation variables} $\delta^{s,\act}$? Idea: Use multiplicative perturbation.

\end{newStuff}

\subsection{Notes}
\iftrue

	\newpage
\subsubsection{Blending, Abstraction}

Assume a set of actions $\Act$.

\paragraph{Autonomy protocol}
The protocol has access to a detailed system model, given as MDP $\MdpInit[_a]$ and a cost function $\rho_a\colon S_a\times\Act\rightarrow\R$. We will sometimes refer to this as \emph{autonomy MDP} and \emph{autonomy cost function}. Assuming the specifications are given, the protocol would be able to compute optimal strategies concerning the performance and adhering to safety. Formally, for a performance specification given as \emph{expected reward property} $\psi=\expRewProp{\kappa}{G}$ and a safety specification given as \emph{probabilistic reachability property} $\varphi=\reachProplT$ with $G,T\subseteq S$, $\kappa\in\R_{\geq 0}$ and $\lambda\in[0,1]$, one can compute a strategy $\sched\in\Sched^{\mdp_a}$ with $\mdp^{\sched}\models\varphi,\psi$ via \emph{multi objective model checking}~\cite{DBLP:journals/lmcs/EtessamiKVY08,DBLP:conf/atva/ForejtKP12}.

\paragraph{Human} 
\subsubsection{Strategy arbitration}
Following~\cite{iturrate-et-al-shared-control-eeg}, the obvious arbitration of the strategies is to choose a value (\eg a function or a real number) that distributes the decisions according to factors such as \emph{safety}, \emph{performance}, or \emph{deviation from the human strategy}. Let $a\in\R$ be such a factor. Given the two (p)MDPs $\pMdpInit[_h]$ and $\MdpInit[_a]$ with $S_h=S_a$ and two (randomized) strategies $\sched_h\in\Sched^{\mdp_h}$ and $\sched_a\in\Sched^{\mdp_a}$. For all states $s\in S_a$ and actions $\act\in\Act$ the arbitrated strategy $\sigma_{ha}\in\Sched^{\mdp_a}$ is then given by
	\begin{align*}
		\sigma_{ha}(s,\alpha)=a\cdot\sched_h(s,\alpha) + (1-a)\cdot\sched_a(s,\alpha) \ .
	\end{align*}
	The situation is more complicated in presence of an abstracted state space as described in the previous paragraph.
\subsection{Correctness issues}

\bigskip
MDP $\mdp_a$ instantiates/refines probmdp $\mdp_h$ and a cost function $\rho_a\colon S\times\Act\rightarrow\R$.

\begin{itemize}
	\item \emph{Human behavior}: .
	\item \emph{Robot behavior}: 
	\item \emph{Comprehensibility of probabilities and cost}: 
	\item \emph{Comprehensibility of the state space}: 	\item \emph{Human's optimality:} Human strategy $\sched_h\colon S\rightarrow\Distr(\Act)$ is $\epsilon$-optimal \wrt $\mdp_h, G, \rho_h$, \ie, for the cost $c'$ induced by $\mdp_h^{\sched_h}$ it holds that $c'=c^*\pm\epsilon$ where $c^*$ is the cost induced by the actual optimal strategy $\sched^*$.
	\item \emph{Robot's optimality:}  Robot strategy $\sched_a$ is optimal \wrt $\mdp_a, G',\rho_a$, \ie, \wrt its own information.
	\item \emph{Blended strategy} $\sched_{hr}\colon S\rightarrow\Distr(\Act)$ depends on confidence modeled by weight $p\in[0,1]$ depending on which information the human had. For each $s\in S$, given $\distFunc_h=\sched_h(s)$ and $\distFunc_a=\sched_a(s)$, we have $\distFunc_{hr}\in\Distr(\Act)$ with $\distFunc_{hr}(\act)=p\cdot\distFunc_a(\act)+(1-p)\cdot\distFunc_h(\act)$ for each $\act\in\Act$. This is similar to~\cite{dragan-et-al-policy-blending}.
	\item \emph{Human feedback:} Add nondeterministic choices to the system which are controlled by the human, \eg, \emph{error signals}. Add action $\mathrm{error}$, which is the only action controlled by human. At critical states, this action means that the human has send a signal and induces a loop to the previous action $\rightsquigarrow$ no further state will be reached (with a certain high probability). Action $\mathrm{nice}$ means that the human has not sent an error signal, thereby ``enforcing'' the previous action.
\end{itemize}

\fi
